# Supplementary material for: Truth Inference on Sparse Crowdsourcing Data with Local Differential Privacy
Source: arXiv:1808.08181 source file (2018-08-24)
Supplement: Supplementary file 1 [file appendix.tex]

\appendix
\section{Error Bound of Algorithm 1}

\begin{theorem}
\label{th:original}
The expected error $E\left[error(\{\hat{a}_j\})\right]$ of estimated truth $\{\hat{a}_j\}$ from Algorithm \ref{alg:estimate} does not exceed \\$\frac{\sqrt{2}}{n\sqrt{\pi}}\sum_{j=1}^{n}\frac{\sum_{W_i\in \overline{W_{j}}}q_i\times\sigma_i}{\sum_{W_i\in \overline{W_{j}}}q_i}$.
\end{theorem}
\vspace{0.2in}
\begin{proof}
\begin{equation}
\label{equ:error_original}
\begin{aligned}
E\left[error(\{\hat{a}_j\})\right]&=E\left[\frac{1}{n}\sum_{j=1}^{n}\left|\mu_j-\hat{a}_j\right|\right]\\
&=\frac{1}{n}\sum_{j=1}^{n}E\left[\left|\mu_j-\hat{a}_j\right|\right]\\
&=\frac{1}{n}\sum_{j=1}^{n}E\left[\left|\mu_j-\frac{\sum_{W_i\in \overline{W_{j}}}{q_i\times a_{i,j}}}{\sum_{W_i\in \overline{W_{j}}} q_i}\right|\right]\\
&=\frac{1}{n}\sum_{j=1}^{n}E\left[\left|\frac{\sum_{W_i\in \overline{W_{j}}}{q_i\times \mu_j}}{\sum_{W_i\in \overline{W_{j}}} q_i}-\frac{\sum_{W_i\in \overline{W_{j}}}{q_i\times a_{i,j}}}{\sum_{W_i\in \overline{W_{j}}} q_i}\right|\right]\\
&=\frac{1}{n}\sum_{j=1}^{n}E\left[\left|\frac{\sum_{W_i\in \overline{W_{j}}}{q_i\times (\mu_j-a_{i,j})}}{\sum_{W_i\in \overline{W_{j}}} q_i}\right|\right]\\
&\le\frac{1}{n}\sum_{j=1}^{n}\frac{\sum_{W_i\in \overline{W_{j}}}q_i\times E\left[\left|\mu_j-a_{i,j}\right|\right]}{\sum_{W_i\in \overline{W_{j}}}q_i}\\
&=\frac{1}{n}\sum_{j=1}^{n}\frac{\sum_{W_i\in \overline{W_{j}}}q_i\times E\left[\left|\mu_j-(\mu_j+\mathcal{N}(0,\sigma_i^2))\right|\right]}{\sum_{W_i\in \overline{W_{j}}}q_i}\\
&=\frac{1}{n}\sum_{j=1}^{n}\frac{\sum_{W_i\in \overline{W_{j}}}q_i\times E\left[\left|\mathcal{N}(0,\sigma_i^2)\right|\right]}{\sum_{W_i\in \overline{W_{j}}}q_i}\\
&=\frac{\sqrt{2}}{n\sqrt{\pi}}\sum_{j=1}^{n}\frac{\sum_{W_i\in \overline{W_{j}}}q_i\times\sigma_i}{\sum_{W_i\in \overline{W_{j}}}q_i}
\end{aligned}
\end{equation}
\end{proof}

\section{Proof of Theorem 4.1}
To prove that the LP mechanism guarantees $\epsilon$-LDP on each answer, it is equivalent to prove that for any pair of answer vectors $\vec{a}_i$ and $\vec{a}_j$ that differ at one element (i.e., the answer of a specific task), $\frac{Pr[\mathcal{L}(\vec{a}_i)=\vec{z}_p]}{Pr[\mathcal{L}(\vec{a}_j)=\vec{z}_p]}\leq e^{\epsilon}$, where $vec{z}_p$ is an arbitrary output answer vector.
Without loss of generality, we assume that they differ at the first element, i.e., $a_{i,1}\neq a_{j,1}$ but $a_{i,k}=a_{j,k}$ for $2\leq k\leq n$.
Also, for the sake of simplicity, we consider $g(\cdot)$ replaces NULL by following a probability mass function $\Omega(v;\Gamma)$ over $\Gamma$. Replacing NULL with a constant $C\in \Gamma$ can be viewed as a special distribution where $\Omega(v;\Gamma)=1$ when $v=C$, and $\Omega(v;\Gamma)=0$ otherwise.
We consider the following three cases.
\begin{itemize}
  \item Case 1. $a_{i,1}\neq NULL$, and $a_{j,1}\neq NULL$. Let $\vec{z}_p\in \Gamma^n$ be any possible answer vector, where $\Gamma$ is the domain of the answers. We have
\begin{equation*}
\begin{aligned}
\frac{P[\mathcal{L}(\vec{a}_i)=\vec{z}_p]}{P[\mathcal{L}(\vec{a}_j)=\vec{z}_p]}&=\frac{\prod_{k=1}^n \exp\left(-\mid z_{pk}-g(a_{i,k})\mid\frac{\epsilon}{|\Gamma|}\right)}{\prod_{k=1}^n \exp\left(-\mid z_{pk}-g(a_{j,k})\mid\frac{\epsilon}{|\Gamma|}\right)}\\
&=\frac{\exp\left(-\mid z_{p1}-a_{i,1}\mid\frac{\epsilon}{|\Gamma|}\right)}{\exp\left(-\mid z_{p1}-a_{j,1}\mid\frac{\epsilon}{|\Gamma|}\right)}\\
 &\leq\exp\left(\frac{\mid a_{i,1} - a_{j,1}\mid}{|\Gamma|}\epsilon\right)\\ 
& \le e^{\epsilon}
\end{aligned}
\end{equation*}

    \item Case 2. $a_{i,1}\neq NULL$, and $a_{j,1}=NULL$. We have 
    \begin{equation*}
\begin{aligned}
\frac{P[\mathcal{L}(\vec{a}_i)=\vec{z}_p]}{P[\mathcal{L}(\vec{a}_j)=\vec{z}_p]}&=\frac{\prod_{k=1}^n \exp\left(-\mid z_{pk}-g(a_{i,k})\mid\frac{\epsilon}{|\Gamma|}\right)}{\prod_{k=1}^n \exp\left(-\mid z_{pk}-g(a_{j,k})\mid\frac{\epsilon}{|\Gamma|}\right)}\\
&=\frac{\exp\left(-\mid z_{p1}-a_{i,1}\mid\frac{\epsilon}{|\Gamma|}\right)}{\sum_{v\in \Gamma} \Omega(v;\Gamma) \exp\left(-|z_{p1}-v|\frac{\epsilon}{|\Gamma|}\right)}\\
&=\frac{\exp\left(-\mid z_{p1}-a_{i,1}\mid\frac{\epsilon}{|\Gamma|}\right)}{\sum_{v\in \Gamma} \Omega(v;\Gamma) \exp\left(-|z_{p1}-v|\frac{\epsilon}{|\Gamma|}\right)}
\end{aligned}
\end{equation*}
For each value $v\in \Gamma$, we have
\begin{equation*}
\frac{\exp\left(-\mid z_{p1}-a_{i,1}\mid\frac{\epsilon}{|\Gamma|}\right)}{\exp\left(-|z_{p1}-v|\frac{\epsilon}{|\Gamma|}\right)}=\exp\left((|z_{p1}-v|-|z_{p1}-a_{i,j}|)\frac{\epsilon}{\Gamma}\right).
\end{equation*}
Obviously, 
\[-|\Gamma|\leq |z_{p1}-v|-|z_{p1}-a_{i,j}|\leq |\Gamma|.\]
Hence, for each $v\in \Gamma$, 
\[e^{-\epsilon}\leq \frac{\exp\left(-\mid z_{p1}-a_{i,1}\mid\frac{\epsilon}{|\Gamma|}\right)}{\exp\left(-|z_{p1}-v|\frac{\epsilon}{|\Gamma|}\right)} \leq e^{\epsilon}.\]
In other words, 
\[\exp\left(-|z_{p1}-v|\frac{\epsilon}{|\Gamma|}\right)\geq e^{-\epsilon} \exp\left(-\mid z_{p1}-a_{i,1}\mid\frac{\epsilon}{|\Gamma|}\right).\]
Therefore, we have 
\begin{equation*}
\begin{aligned}
& \frac{\exp\left(-|z_{p1}-a_{i,1}|\frac{\epsilon}{|\Gamma|}\right)}{\sum_{v\in \Gamma} \Omega(v;\Gamma) \exp\left(-|z_{p1}-v|\frac{\epsilon}{|\Gamma|}\right)}\\
\leq & \frac{\exp\left(-|z_{p1}-a_{i,1}|\frac{\epsilon}{|\Gamma|}\right)}{\sum_{v\in \Gamma} \Omega(v;\Gamma) e^{-\epsilon}\exp\left(-|z_{p1}-a_{i,1}|\frac{\epsilon}{|\Gamma|}\right)} \\
= & \frac{e^{\epsilon}}{\sum_{v\in \Gamma} \Omega(v;\Gamma)} \\
= & e^{\epsilon}
\end{aligned}
\end{equation*}

  \item Case 3. $a_{i,1}= NULL$, and $a_{j,1}\neq NULL$. This is analogous to Case 2. We have
    \begin{equation*}
  \begin{aligned}
  \frac{P[\mathcal{L}(\vec{a_i})=\vec{z_p}]}{P[\mathcal{L}(\vec{a_j})=\vec{z_p}]}&=\frac{\prod_{k=1}^n \exp\left(-\mid z_{pk}-g(a_{i,k})\mid\frac{\epsilon}{|\Gamma|}\right)}{\prod_{k=1}^n \exp\left(-\mid z_{pk}-g(a_{j,k})\mid\frac{\epsilon}{|\Gamma|}\right)}\\
&=\frac{\sum_{v\in \Gamma} \Omega(v;\Gamma) \exp\left(-|z_{p1}-v|\frac{\epsilon}{|\Gamma|}\right)}{\exp\left(-\mid z_{p1}-a_{j,1}\mid\frac{\epsilon}{|\Gamma|}\right)}\\
&\leq \frac{\sum_{v\in \Gamma} \Omega(v;\Gamma) e^{\epsilon}\exp\left(-\mid z_{p1}-a_{j,1}\mid\frac{\epsilon}{|\Gamma|}\right)}{\exp\left(-\mid z_{p1}-a_{j,1}\mid\frac{\epsilon}{|\Gamma|}\right)}\\
& = \sum_{v\in \Gamma} \Omega(v;\Gamma) e^{\epsilon}\\
& = e^{\epsilon}
\end{aligned}
\end{equation*}
\end{itemize}
Based on the discussion of three cases, it can be concluded that LP mechanism guarantees $\epsilon$-LDP.

\section{Proof of Theorem 4.2}
Based on the proof in Equation (\ref{equ:error_original}), we just need to calculate $E\left[\left|\mu_j-a_{i,j}\right|\right]$ in line 6:

\resizebox{0.34\textwidth}{!}{
\begin{minipage}{\linewidth}
\begin{equation}
\begin{aligned}
&E\left[\left|\mu_j-a_{i,j}\right|\right]\\
=&E\left[\left|\mu_j-(1-s_i) \left(\Omega(\Gamma)+Lap\left(\frac{|\Gamma|}{\epsilon}\right)\right)-s_i\left(\mu_j+\mathcal{N}(0,\sigma_i)+Lap\left(\frac{|\Gamma|}{\epsilon}\right)\right)\right|\right]\\
=&E\left[\left|(1-s_i+s_i)\mu_j-(1-s_i) \left(\Omega(\Gamma)+Lap\left(\frac{|\Gamma|}{\epsilon}\right)\right)-s_i\left(\mu_j+\mathcal{N}(0,\sigma_i)+Lap\left(\frac{|\Gamma|}{\epsilon}\right)\right)\right|\right]\\
=&E\left[\left|(1-s_i) \left(\mu_j-\Omega(\Gamma)-Lap\left(\frac{|\Gamma|}{\epsilon}\right)\right)-s_i\left(\mu_j+\mathcal{N}(0,\sigma_i)+Lap\left(\frac{|\Gamma|}{\epsilon}\right)-\mu_j\right)\right|\right]\\
\le&(1-s_i)E\left[\left|\mu_j-\Omega(\Gamma)-Lap\left(\frac{|\Gamma|}{\epsilon}\right)\right|\right]+s_iE\left[\left|\mathcal{N}(0,\sigma_i)+Lap\left(\frac{|\Gamma|}{\epsilon}\right)\right|\right]\\
\le&(1-s_i)\left(E\left[\left|\mu_j-\Omega(\Gamma)\right|\right]+\frac{|\Gamma|}{\epsilon}\right)+s_i\left(\sigma_i\sqrt{\frac{2}{\pi}}+\frac{|\Gamma|}{\epsilon}\right)\\
=&(1-s_i)\left(\phi_{\mu_j}(\Gamma)+\frac{|\Gamma|}{\epsilon}\right)+s_i\left(\sigma_i\sqrt{\frac{2}{\pi}}+\frac{|\Gamma|}{\epsilon}\right)\\
=&e_{i,j}^{LP}
\end{aligned}
\end{equation}
\end{minipage}
}

where $\phi_{\mu_j}(\Gamma)=E\left[\left|\mu_j-\Omega(\Gamma)\right|\right]$. Specially, when $\Omega(\Gamma)=c$ is a constant $c$, we have \[\phi_{\mu_j}(\Gamma)=E\left[\left|\mu_j-\Omega(\Gamma)\right|\right]=|\mu_j-c|\]when $\Omega(\Gamma)=U(\Gamma)$ is a uniform distribution, we have \[\phi_{\mu_j}(\Gamma)=E\left[\left|\mu_j-\Omega(\Gamma)\right|\right]=\frac{(t-\mu_j)^2+(\mu_j-s)^2}{2(t-s)}\], where $s,t\in\Gamma$ is the minimum and maximum value in $\Gamma$.

Substitute the result above into line 6 of equation (\ref{equ:error_original}), we have:
\begin{equation*}
\begin{aligned}
E\left[Error(\{\hat{a}_j\})\right]&\le\frac{1}{n}\sum_{j=1}^{n}\frac{\sum_{W_i\in \overline{W_{j}}}q_i\times E\left[\left|\mu_j-a_{i,j}\right|\right]}{\sum_{W_i\in \overline{W_{j}}}q_i}\\
&=\frac{1}{n}\sum_{j=1}^{n}\frac{\sum_{W_i\in \overline{W_{j}}}q_i\times e_{i,j}^{LP}}{\sum_{W_i\in \overline{W_{j}}}q_i}\\
\end{aligned}
\end{equation*}
Since LP will fill all the NULL values and $\sum_{i=1}^m q_i=1$, therefore:
\begin{equation*}
\begin{aligned}
&=\frac{1}{n}\sum_{j=1}^{n}\frac{\sum_{i=1}^{m}q_i\times e_{i,j}^{LP}}{\sum_{i=1}^{m}q_i}\\
&=\frac{1}{n}\sum_{j=1}^{n}\sum_{i=1}^{m}q_i\times e_{i,j}^{LP}
\end{aligned}
\end{equation*}\qed

%-------------------------------------

\section{Proof of Theorem 4.4}
Based on the proof in Equation (\ref{equ:error_original}), we just need to calculate $E\left[\left|\mu_j-a_{i,j}\right|\right]$ in line 6:

\resizebox{0.35\textwidth}{!}{
\begin{minipage}{\linewidth}
\begin{equation}
\begin{aligned}
&E\left[\left|\mu_j-a_{i,j}\right|\right]\\
=&E\left[\left|\mu_j-(1-s_i)Y_{NULL}-\sum_{x\in\Gamma}s_iP(x)Y_x\right|\right]\\
=&E\left[\left|\left(1-s_i+\sum_{x\in\Gamma}s_i\mathcal{N}(x;\mu_j,\sigma_i)\right)\mu_j-(1-s_i)Y_{NULL}-\sum_{x\in\Gamma}s_i\mathcal{N}(x;\mu_j,\sigma_i)Y_x\right|\right]\\
=&E\left[\left|(1-s_i)(\mu_j-Y_{NULL})+\sum_{x\in\Gamma}s_i\mathcal{N}(x;\mu_j,\sigma_i)(\mu_j-Y_x)\right|\right]\\
\le&E\left[\left|(1-s_i)(\mu_j-Y_{NULL})\right|\right]+E\left[\left|\sum_{x\in\Gamma}s_i\mathcal{N}(x;\mu_j,\sigma_i)(\mu_j-Y_x)\right|\right]\\
\le&(1-s_i)E\left[\left|\mu_j-Y_{NULL}\right|\right]+\sum_{x\in\Gamma}s_i\mathcal{N}(x;\mu_j,\sigma_i)E\left[\left|\mu_j-Y_x\right|\right]\\
=&(1-s_i)\left|\mu_j-\sum_{y\in\Gamma}y\frac{1}{e^{\epsilon}+|\Gamma|}\right|+\sum_{x\in\Gamma}s_i\mathcal{N}(x;\mu_j,\sigma_i)\left|\mu_j-\sum_{y\in\Gamma}yP(y|x)\right|\\
=&e_{i,j}^{RR}
\end{aligned}
\end{equation}
\end{minipage}
}

where $Y_{NULL}$ and $Y_x$ are the distribution of observing $a_{i,j}$ as a normal value when the original value is NULL or $x$.

Substitute the result above into line 6 of equation (\ref{equ:error_original}), we have:
\begin{equation*}
\begin{aligned}
E\left[Error(\{\hat{a}_j\})\right]&\le\frac{1}{n}\sum_{j=1}^{n}\frac{\sum_{W_i\in \overline{W_{j}}}q_i\times E\left[\left|\mu_j-a_{i,j}\right|\right]}{\sum_{W_i\in \overline{W_{j}}}q_i}\\
&=\frac{1}{n}\sum_{j=1}^{n}\frac{\sum_{W_i\in \overline{W_{j}}}q_i\times e_{i,j}^{RR}}{\sum_{W_i\in \overline{W_{j}}}q_i}
\end{aligned}
\end{equation*}\qed

%------------------------------------

\section{Proof of Theorem 5.2}
Based on the proof in Equation (\ref{equ:error_original}), we just need to calculate $E\left[\left|\mu_j-a_{i,j}\right|\right]$ in line 6:

\resizebox{0.30\textwidth}{!}{
\begin{minipage}{\linewidth}
\begin{equation}
\begin{aligned}
&E\left[\left|\mu_j-a_{i,j}\right|\right]\\
=&E\left[\left|\mu_j-\frac{1}{s_i+e^{\epsilon_1}(1-s_i)}\left(s_i\left(\mathcal{N}(\mu_j,\sigma_i)+Lap\left(\frac{|\Gamma|}{\epsilon_2}\right)\right)-e^{\epsilon_1}(1-s_i)\left(U(\Gamma)+Lap\left(\frac{|\Gamma|}{\epsilon_2}\right)\right)\right)\right|\right]\\
=&E\left[\left|\frac{1}{s_i+e^{\epsilon_1}(1-s_i)}\left(s_i\left(\mu_j-\mathcal{N}(\mu_j,\sigma_i)-Lap\left(\frac{|\Gamma|}{\epsilon_2}\right)\right)+e^{\epsilon_1}(1-s_i)\left(\mu_j-U(\Gamma)-Lap\left(\frac{|\Gamma|}{\epsilon_2}\right)\right)\right)\right|\right]\\
\le&\frac{1}{s_i+e^{\epsilon_1}(1-s_i)}\left(s_iE\left[\left|\mu_j-\mathcal{N}(\mu_j,\sigma_i)-Lap\left(\frac{|\Gamma|}{\epsilon_2}\right)\right|\right]+e^{\epsilon_1}(1-s_i)E\left[\left|\mu_j-U(\Gamma)-Lap\left(\frac{|\Gamma|}{\epsilon_2}\right)\right|\right]\right)\\
\le&\frac{1}{s_i+e^{\epsilon_1}(1-s_i)}\left(s_i\left(\sigma_i\sqrt{\frac{2}{\pi}}+\frac{|\Gamma|}{\epsilon}\right)+e^{\epsilon_1}(1-s_i)\left(E\left[\left|\mu_j-U(\Gamma)\right|\right]+\frac{|\Gamma|}{\epsilon_2}\right)\right)\\
=&\frac{1}{s_i+e^{\epsilon_1}(1-s_i)}\left(s_i\left(\sigma_i\sqrt{\frac{2}{\pi}}+\frac{|\Gamma|}{\epsilon}\right)+e^{\epsilon_1}(1-s_i)\left(\psi_{\mu_j}(\Gamma)+\frac{|\Gamma|}{\epsilon_2}\right)\right)\\
=&e_{i,j}^{RR+LP}
\end{aligned}
\end{equation}
\end{minipage}
}

where
\begin{equation*}
\psi_{\mu_j}(\Gamma)=E\left[\left|\mu_j-U(\Gamma)\right|\right]=\frac{(t-\mu_j)^2+(\mu_j-s)^2}{2(t-s)}
\end{equation*} $s,t\in\Gamma$ are the maximum and minimum value of the answer domain.

Substitute the result above into line 6 of equation (\ref{equ:error_original}), we have:
\begin{equation*}
\begin{aligned}
E\left[Error(\{\hat{a}_j\})\right]&\le\frac{1}{n}\sum_{j=1}^{n}\frac{\sum_{W_i\in \overline{W_{j}}}q_i\times E\left[\left|\mu_j-a_{i,j}\right|\right]}{\sum_{W_i\in \overline{W_{j}}}q_i}\\
&=\frac{1}{n}\sum_{j=1}^{n}\frac{\sum_{W_i\in \overline{W_{j}}}q_i\times e_{i,j}^{RR+LP}}{\sum_{W_i\in \overline{W_{j}}}q_i}
\end{aligned}
\end{equation*}\qed

%------------------------------------

\section{Proof of Theorem 6.2}
Since we have:
\begin{equation}
\nabla_{\vec{u_i}}L_{DP}(\vec{a_i}, \vec{u_i}, V)=2\vec{\eta_i}-\sum_{j=1}^n 2\vec{v_j}(a_{i,j}-\vec{u_i} \vec{v_j})=0
\end{equation}

We can infer that
\begin{equation}
\begin{aligned}
\vec{\eta_i}-\sum_{j=1}^n \vec{v_j}(a_{ij}-\vec{u_i} \vec{v_j})&=0\\
\sum_{j=1}^{n}\vec{v}_j (\vec{u}_i\vec{v}_j)&=\sum_{j=1}^{n}\vec{v}_j a_{i,j}-\vec{\eta}_i
\end{aligned}
\end{equation}

furthermore, 
\begin{equation}
\begin{aligned}
\label{equ:leftnright}
\sum_{j=1}^{n}\vec{v}_j\left|\mu_j-\vec{u}_i\vec{v}_j\right|&=\left|\sum_{j=1}^{n}\vec{v}_j\mu_j-\sum_{j=1}^{n}\vec{v}_j(\vec{u}_i\vec{v}_j)\right|\\
&=\left|\sum_{j=1}^{n}\vec{v}_j\mu_j-\sum_{j=1}^{n}\vec{v}_j a_{i,j}+\vec{\eta}_i\right|\\
&=\left|\sum_{j=1}^{n}\vec{v}(\mu_j-a_{i,j})+\vec{\eta}_i\right|\\
&=\left|\sum_{j=1}^{n}\vec{v}\mathcal{N}(0,\sigma_i)+\vec{\eta}_i\right|
% &\le\left|\sum_{j=1}^{n}\vec{v}_j\mu_j\right|+\left|\sum_{j=1}^{n}\vec{v}_j a_{i,j}\right|+|\eta_i|\\
% &=\sum_{j=1}^{n}\vec{v}_j\mu_j+\sum_{j=1}^{n}\vec{v}_j |\mu_j+\mathcal{N}(0,\sigma_j)|+|\eta_i|
\end{aligned}
\end{equation}

\begin{equation}
\begin{aligned}
\label{equ:left}
E\left[\sum_{j=1}^{n}\vec{v}_j\left|\mu_j-\vec{u}_i\vec{v}_j\right|\right]&=\sum_{j=1}^{n}E[\vec{v}_j]E[|\mu_j-\vec{u}_i\vec{v}_j|]
\end{aligned}
\end{equation}

\begin{equation}
\begin{aligned}
\label{equ:right}
E\left[\left|\sum_{j=1}^{n}\vec{v}\mathcal{N}(0,\sigma_i)+\vec{\eta}_i\right|\right]&\le\sum_{j=1}^{n}E[\vec{v}_j]E[|\mathcal{N}(0,\sigma_i)|]+E[|\vec{\eta}_i|]\\
&=\sum_{j=1}^{n}E[\vec{v}_j]\sigma_i\sqrt{\frac{2}{\pi}}+E[|\vec{\eta}_i|]
\end{aligned}
\end{equation}

Because $\left\|\vec{v}_j\right\|=1$ and it's a positive vector generated by uniform distribution, thus $E[\vec{v}_j]=\{\frac{1}{d}\}_d$. For $\vec{\eta}_i$, each dimension of $\eta_i$ is generated by Laplace distribution, therefore $E[|\vec{\eta}_i|]=\{E\left[\left|Lap\left(\frac{|\Gamma|}{\epsilon}\right)\right|\right]\}_d=\{\frac{|\Gamma|}{\epsilon}\}_d$. According to equation (\ref{equ:leftnright}), equation (\ref{equ:left}) and (\ref{equ:right}) are equal. Then if we focus on any specific dimension, we can infer that 
\begin{equation*}
\begin{aligned}
\frac{1}{d}\sum_{j=1}^{n}E[|\mu_j-\vec{u}_i\vec{v}_j|]&\le\frac{n}{d}\sqrt{\frac{2}{\pi}}+\frac{|\Gamma|}{\epsilon}\\
\sum_{j=1}^{n}E[|\mu_j-\vec{u}_i\vec{v}_j|]&\le n\sqrt{\frac{2}{\pi}}+d\frac{|\Gamma|}{\epsilon}
\end{aligned}
\end{equation*}

The expected error of truth inference is:
\begin{equation*}
\begin{aligned}
E\left[Error(\{\hat{a}_j\})\right]&=E\left[\frac{1}{n}\sum_{j=1}^{n}\left|\mu_j-\hat{a}_j\right|\right]\\
&=\frac{1}{n}\sum_{j=1}^{n}E\left[\left|\mu_j-\hat{a}_j\right|\right]\\
&=\frac{1}{n}\sum_{j=1}^{n}E\left[\left|\mu_j-\frac{\sum_{i=1}^{m}{q_i\times \vec{u}_i\vec{v}_j}}{\sum_{i=1}^{m} q_i}\right|\right]\\
&=\frac{1}{n}\sum_{j=1}^{n}E\left[\left|\frac{\sum_{i=1}^{m}{q_i\times \mu_j}}{\sum_{i=1}^{m} q_i}-\frac{\sum_{i=1}^{m}{q_i\times \vec{u}_i\vec{v}_j}}{\sum_{i=1}^{m} q_i}\right|\right]\\
&=\frac{1}{n}\sum_{j=1}^{n}E\left[\left|\frac{\sum_{i=1}^{m}{q_i\times (\mu_j-\vec{u}_i\vec{v}_j)}}{\sum_{i=1}^{m} q_i}\right|\right]\\
&\le\frac{1}{n}\sum_{j=1}^{n}\frac{\sum_{i=1}^{m}q_i\times E\left[\left|\mu_j-\vec{u}_i\vec{v}_j\right|\right]}{\sum_{i=1}^{m}q_i}\\
&=\frac{1}{n}\sum_{j=1}^{n}\sum_{i=1}^{m}q_i\times E\left[\left|\mu_j-\vec{u}_i\vec{v}_j\right|\right]\\
&\text{switch the order of sum}\\
&=\frac{1}{n}\sum_{i=1}^{m}\sum_{j=1}^{n}q_i\times E\left[\left|\mu_j-\vec{u}_i\vec{v}_j\right|\right]\\
&\text{Let $\tilde{q}=max\{q_i\}=O(1/m)$}\\
&\le\frac{1}{n}\sum_{j=1}^{n}\sum_{i=1}^{m} \tilde{q}E\left[\left|\mu_j-\vec{u}_i\vec{v}_j\right|\right]\\
&=\frac{\tilde{q}}{n}\sum_{i=1}^{m}\sum_{j=1}^{n} E\left[\left|\mu_j-\vec{u}_i\vec{v}_j\right|\right]\\
&\le\frac{\tilde{q}}{n}\sum_{i=1}^{m}\left(n\sqrt{\frac{2}{\pi}}+d\frac{|\Gamma|}{\epsilon}\right)\\
&=\tilde{q}m\left(\sqrt{\frac{2}{\pi}}+\frac{d|\Gamma|}{n\epsilon}\right)
\end{aligned}
\end{equation*}\qed

\subsection{Experimental results with various privacy budget on large dataset}
%%%%%%%%%%%%%%%%%%%%%%%include in the full paper %%%%%%%%%%%%%%%%%%%%%%%

\begin{figure*}[!htbp]
\begin{center}
\begin{tabular}{@{}c@{}c@{}c@{}}
	\includegraphics[width=0.33\textwidth]{./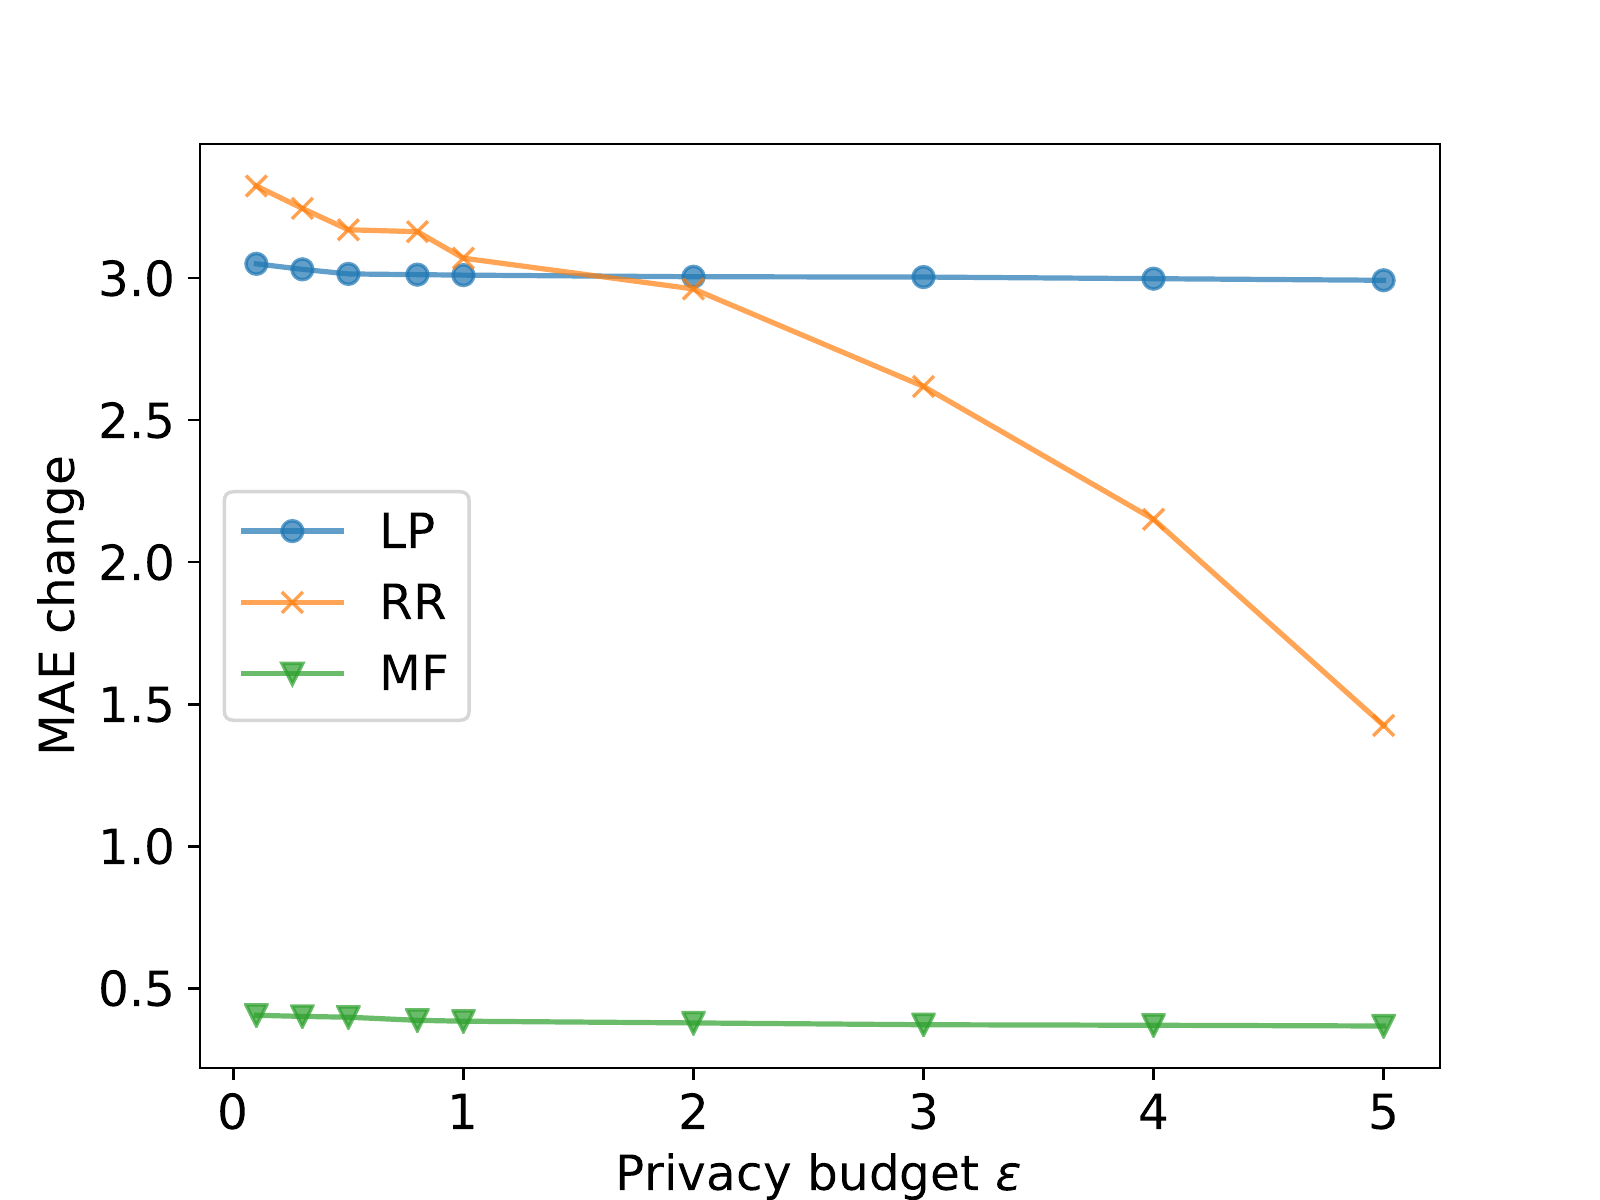} 
	&
	\includegraphics[width=0.33\textwidth]{./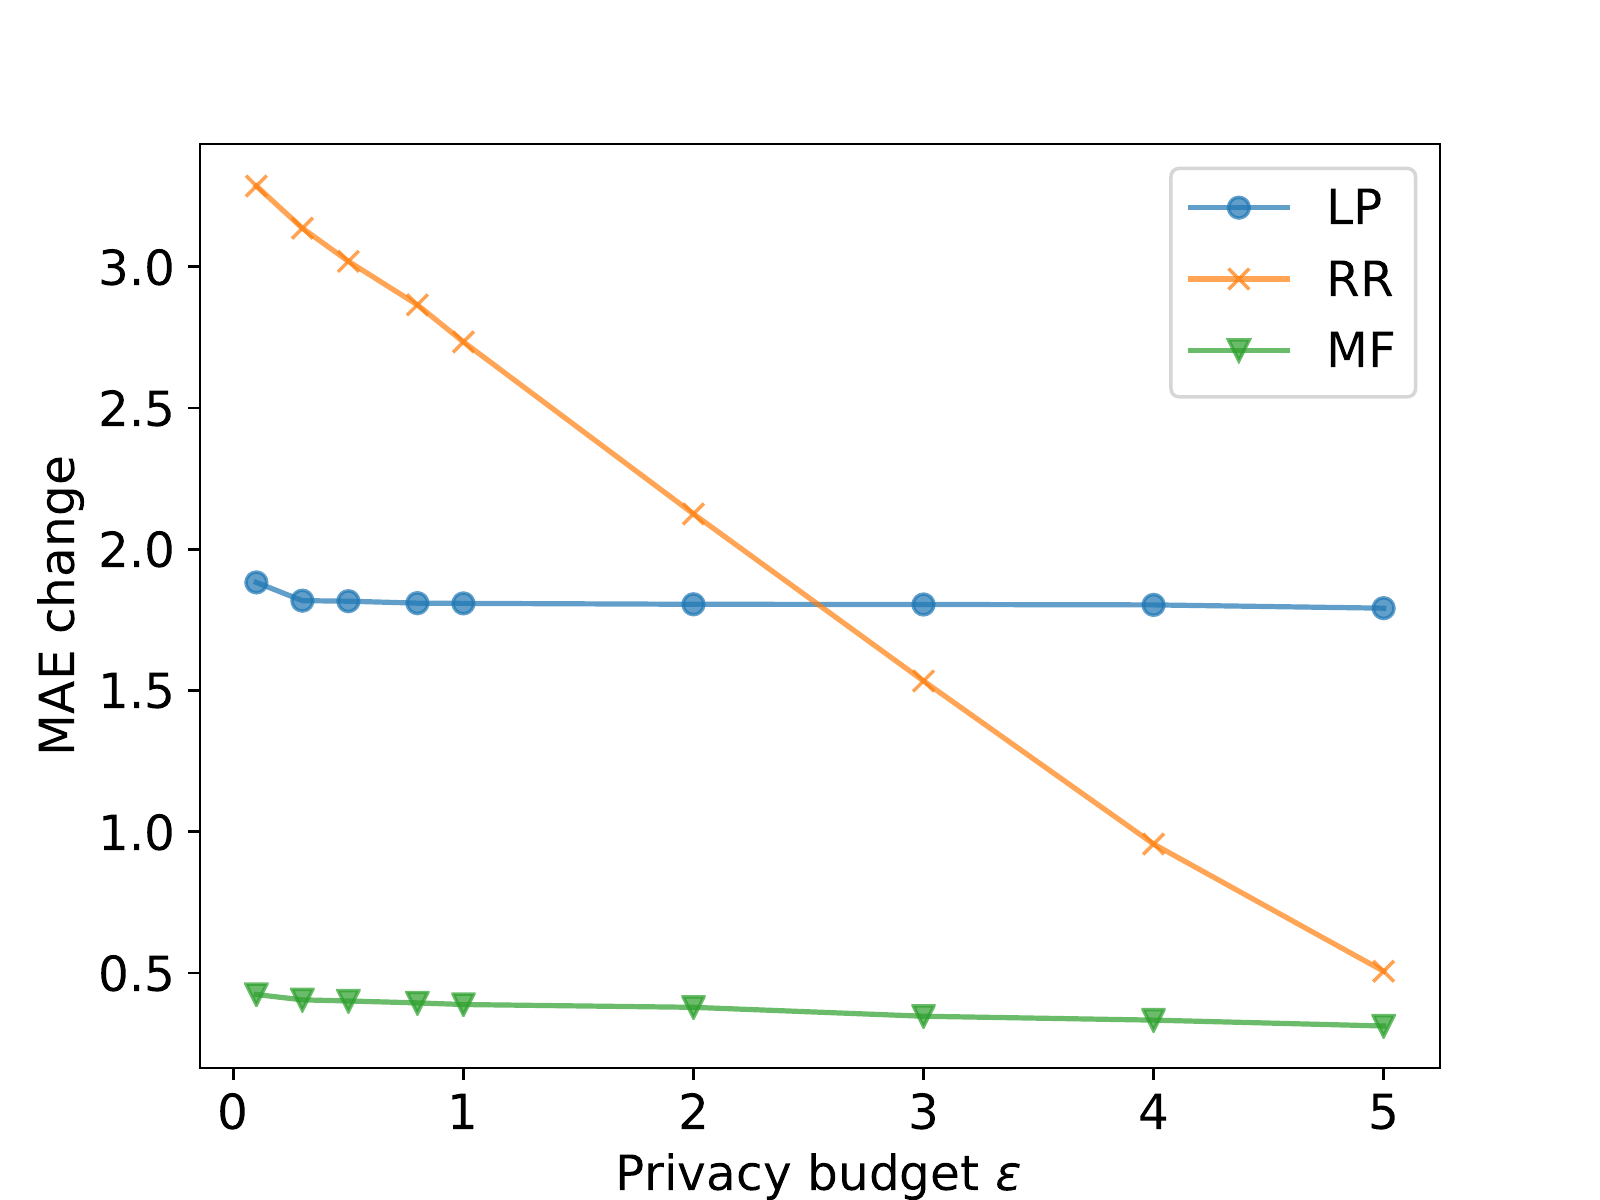}
	&
	\includegraphics[width=0.33\textwidth]{./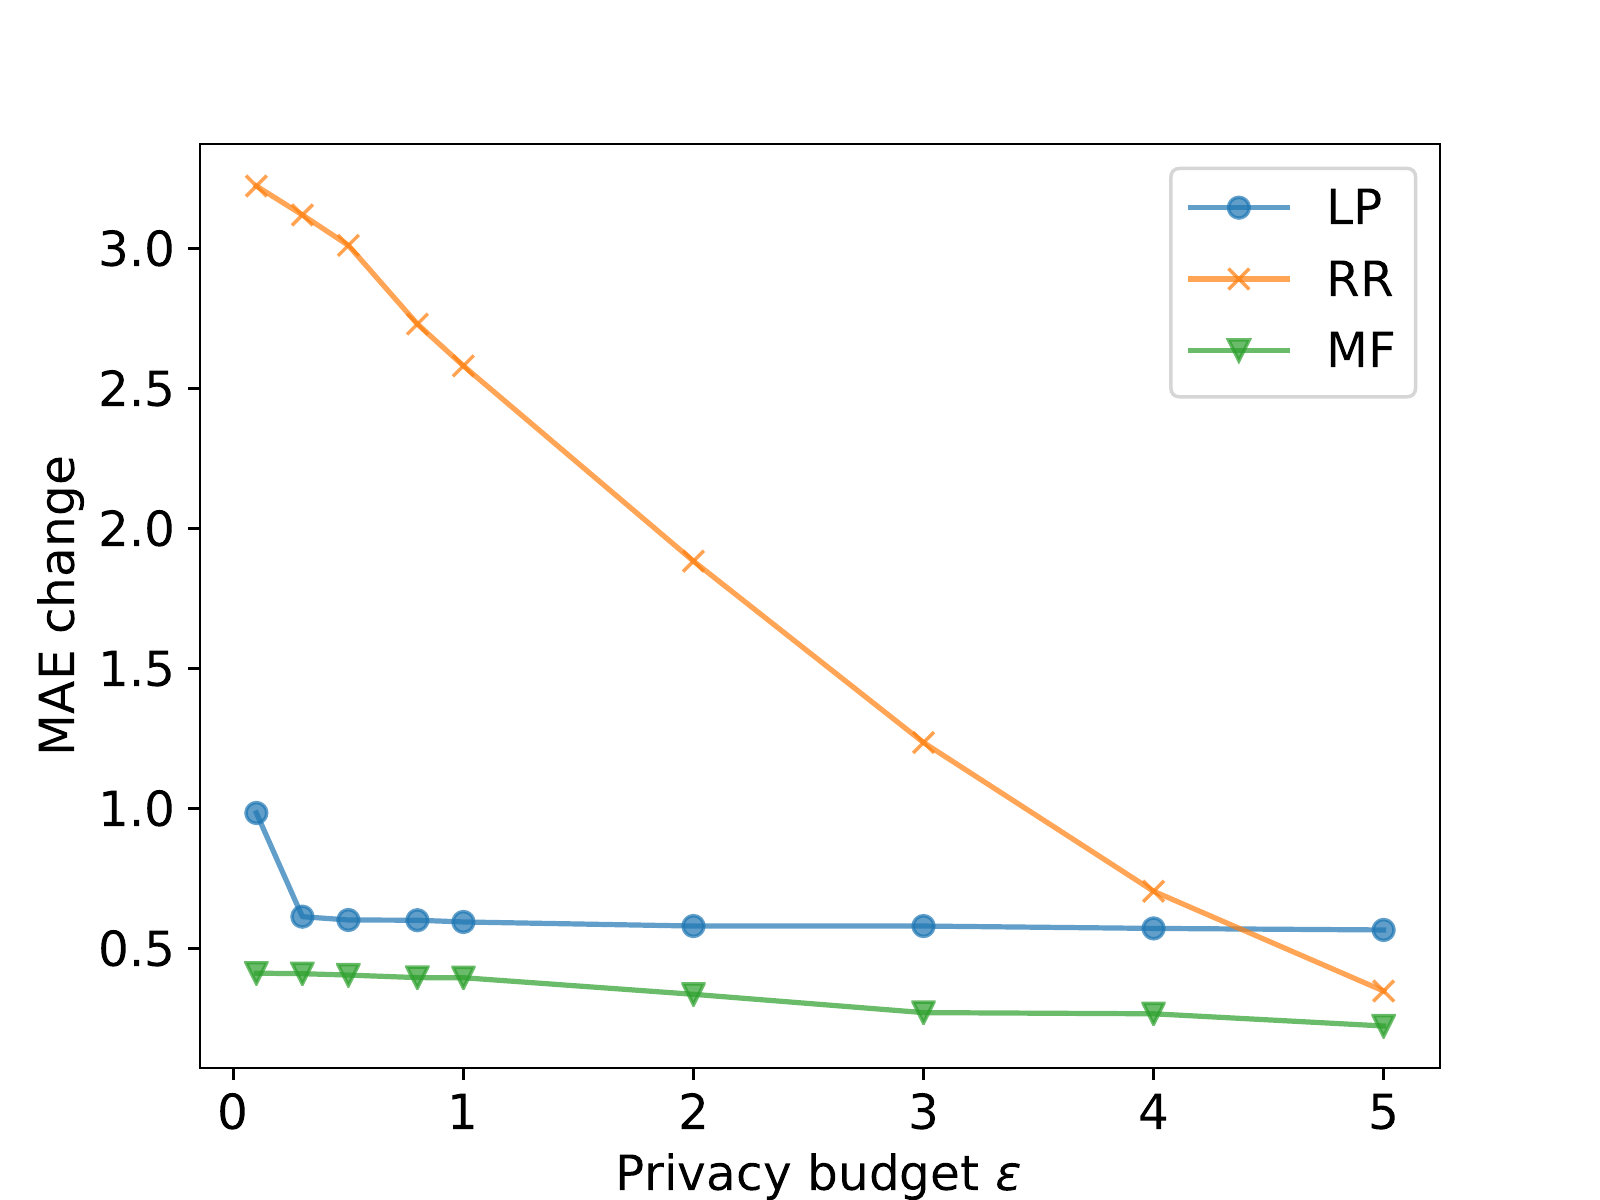}
	\\
	{\scriptsize(a) sparsity$=0.9$, truth distribution $\mathcal{N}(0,1)$}
	&
	{\scriptsize(b) sparsity$=0.5$, truth distribution $\mathcal{N}(0,1)$}
	&
	{\scriptsize(c) sparsity$=0.1$, truth distribution $\mathcal{N}(0,1)$}
	\\
    \includegraphics[width=0.33\textwidth]{./Figures/m10000n1000den0_10skew5_comp4_varyEpsilon.pdf} 
	&
	\includegraphics[width=0.33\textwidth]{./Figures/m10000n1000den0_50skew5_comp4_varyEpsilon.pdf}
	&
	\includegraphics[width=0.33\textwidth]{./Figures/m10000n1000den0_90skew5_comp4_varyEpsilon.pdf}
	\\
	{\scriptsize(d) sparsity$=0.9$, truth distribution $\mathcal{N}(4,1)$}
	&
	{\scriptsize(e) sparsity$=0.5$, truth distribution $\mathcal{N}(4,1)$}
	&
	{\scriptsize(f) sparsity$=0.1$, truth distribution $\mathcal{N}(4,1)$}
\end{tabular}
\vspace{-0.1in}
\caption{\small \label{fig:ae_wrt_epsilon_10000} Accuracy of truth inference w.r.t. different privacy budget $\epsilon$ (10000 workers and 1000 tasks).}
\end{center}
\end{figure*}
